# Supplementary material for: Sample Complexity of Robust Reinforcement Learning with a Generative Model
Source: arXiv:2112.01506 source file (2022-05-14)
Supplement: Supplementary file 2 [file 06-Appendix-old.tex]

\appendix
\onecolumn
\section*{\redtext{Old Appendix}}

\section{Useful vanilla results}
In this section we state a few existing celebrated results in the literature that are useful in our analysis.

\begin{lemma}[Hoeffding's inequality \hspace{-0.1cm}\text{\cite[Theorem 2.2.6]{vershynin2018high}}] \label{lem:hoeffding_ineq}
Let $X_1,\cdots, X_T$ be independent random variables. Assume that $X_t \in [m_t, M_t]$ for every $t$ with $M_t > m_t$. Then, for any $\epsilon > 0$, we have \[ \pr \left( \sum_{t=1}^T (X_t - \E[X_t]) \geq \epsilon \right) \leq \exp\left( -\frac{2\epsilon^2}{\sum_{t=1}^T (M_t - m_t)^2} \right). \]
\end{lemma}

\begin{lemma}[Kantorovich-Rubinstein Theorem \hspace{-0.1cm}\text{\cite[Theorem 11.8.2]{dudley2002real}}] \label{lem:kantorovich-rubinstein-theorem}
For any separable metric space $(S,d)$ and any two probability laws $P$ and $Q$ in $\Delta^{|S|}$ we have \[ \inf_{\nu\in M(P,Q)} \int_{(x,y)\in S\times S} d(x,y)\, \dd\nu(x,y) = \sup_{f:\|f\|_{*} \leq 1} \left|\int f\,\dd(P-Q) \right|, \] where $\|f\|_{*} := \sup\{ |f(x)-f(y)|/d(x,y):\, x\neq y \text{ in } S\}$.
\end{lemma}

\section{Proof of Theorems \ref{thm:revi-guarantee-l1-Wasserstein}-\ref{thm:revi-guarantee-kul-lieb}}

We now start by restating the supporting results and provide their proofs.

Now restating Lemma \ref{lem:hoeffding_concentration}.
\begin{lemma}%\label{lem:hoeffding_concentration}
	Consider any value function $V\in \R^{|\Ss|}$ bounded as $\|V\| \leq V_{\text{max}}$ for some $V_{\text{max}}>0$. Under Assumption 1, \[ \max_{(s,a)} |{P^o_{s,a}} V -  \widehat{P}_{s,a} V | \leq V_{\text{max}} \sqrt{\frac{\log(2|\Ss||\Aa|/\delta)}{2N}}\] holds with probability at least $1-\delta$.
\end{lemma}
\begin{proof}
	Fix any $(s,a)$ pair. %Let the empirical estimate $\widehat{P}$ be built by taking $N(s,a)$ samples for this pair. $N(s,a)= N$ from Assumption 1. 
	Consider an $|\Ss|$-length discrete random variable $X$ taking value $V(j)$ with probability $P^o_{s,a}(j)$ for all $j\in\{1,2,\cdots,|\Ss|\}$. From Hoeffding's inequality - i.e. Lemma \ref{lem:hoeffding_ineq} - we have \begin{align*} &\pr \{P^o_{s,a} V -  \widehat{P}_{s,a} V  \geq \epsilon \} \leq \exp(-2  N \epsilon^2/V^2_{\text{max}}) \text{ and }\\
	&\pr \{\widehat{P}_{s,a} V -  P^o_{s,a} V  \geq \epsilon \} \leq \exp(-2  N \epsilon^2/V^2_{\text{max}}).\end{align*} Choosing \[ \epsilon = V_{\text{max}} \sqrt{\frac{\log(2|\Ss||\Aa|/\delta)}{2N}}, \] we get \[ \pr \{|P^o_{s,a} V -  \widehat{P}_{s,a} V | \geq V_{\text{max}} \sqrt{\frac{\log(2|\Ss||\Aa|/\delta)}{2N}} \} \leq \frac{\delta}{|\Ss||\Aa|}.  \] Now, by union bound, we get \begin{align*}
	&\pr \{ \max_{(s,a)} |P^o_{s,a} V -  \widehat{P}_{s,a} V | \geq V_{\text{max}} \sqrt{\frac{\log(2|\Ss||\Aa|/\delta)}{2N}} \} \leq \sum_{s,a} \pr \{|P^o_{s,a} V -  \widehat{P}_{s,a} V | \geq V_{\text{max}} \sqrt{\frac{\log(2|\Ss||\Aa|/\delta)}{2N}} \} \hspace{-0.05cm}\leq\hspace{-0.05cm} \delta. 
	\end{align*} The proof is now complete.
\end{proof}

% From \cite[Exercise 5.5 and Lemma 5.13]{van2014probability} we have the following result.
% \begin{lemma}[Covering Number of $\V$]
% \label{por:covering_num}
% Let $\V$ denote a bounded class of functions mapping from $\Ss$ to $\R$, that is, \[ \V = \{V\in \R^{|\Ss|}~:~ \|V\| \leq 1/(1-\gamma)\}.\] Let $\N_\eta$ be the $\eta$-covering number of $\V$ with respect to the distance metric $dist(V,V') = \sup_{s\in\Ss} |V(s)-V'(s)|$ for some fixed $\eta\in (0,1).$ Let $\N_\V (\subseteq \V)$ be its corresponding minimal $\eta$-cover. Then we have 
% 	$$
% 	\log \N_\eta  \leq |\Ss| \cdot \log \left( \frac{3}{(1-\gamma)\eta}  \right) .	$$
% \end{lemma}

% \begin{lemma}[\hspace{-0.1cm}\text{\cite[Lemma 4.3]{iyengar2005robust}}]
%     For an $\ell_1$-uncertainty set $\Pp$ centered with distribution $Q\in\Delta^{|\Ss|}$, \begin{align*} &\sigma_{{\Pp}} (V) = QV + \max_{\mu: 0 \leq \mu \leq V} \bigg( -Q \mu  + \frac{c_r}{2} (\min_{s} (V_\mu(s)) - \max_{s} (V_\mu(s))) \bigg), 
%     \end{align*} where $V_\mu(s)=V(s)-\mu(s)$ for all $s\in\Ss$.
% \end{lemma}

Now restating Lemma \ref{lem:wasserstein_inner_prob}.
\begin{lemma}
    Consider any ${V}\in (0,1/(1-\gamma)]^{|\Ss|}$. For the Wasserstein uncertainty set $\Pp$ centered with distribution $Q\in\Delta^{|\Ss|}$, \begin{align*} &\sigma_{{\Pp}} (V) = QV + \max_{\mu:0 \leq \mu \leq V} \big( -Q\mu  - \min\{\| V-\mu-\alpha_\mu\mathbbm{1} \|_2^2, {c_r}/{(1-\gamma)}\}\big),
    \end{align*} where $\alpha_\mu = (1/|\Ss|)\sum_{s\in\Ss}(V(s)-\mu(s)).$
\end{lemma}
\begin{proof}
    Recall the Wasserstein uncertainty set definition \[ \Pp =  \{ P \in \Delta^{|\Ss|} ~:~ \inf_{\nu\in M(P,Q)} \int_{(x,y)\in\Ss\times\Ss} 2\, \dd\nu(x,y) \leq c_r \}. \] From the Kantorovich-Rubinstein theorem (i.e. Lemma \ref{lem:kantorovich-rubinstein-theorem}), taking $d$ to be an indicator metric - $d(x,y)=2\cdot\mathbbm{1}(x\neq y)$ - and $f=(1-\gamma)\widetilde{V}$, we can write the above as
    \[ \Pp =  \{ P \in \Delta^{|\Ss|} ~:~ \sup_{\widetilde{V}:\|\widetilde{V}\|_{*} \leq 1/(1-\gamma)} |P\widetilde{V} - Q\widetilde{V}| \leq c_r/(1-\gamma) \}. \] Recall that $\|\widetilde{V}\|_{*} = \sup \{ |\widetilde{V}(x)-\widetilde{V}(y)|/2:\, x\neq y \text{ in }\Ss \}$. We note that the functional metric in the reformulation of $\Pp$ is referred to as an Integral Probability metric.
    Letting $y(s) = P(s) - Q(s)$ for all $s\in\Ss$, we have \begin{align*} \sigma_{{\Pp}} (V) = QV + &\min && \hspace{-2cm} y^\top V  \\
    &\text{s.t.} &&\hspace{-2cm}\sum_{s\in\Ss} y(s) = 0, y\geq -Q, \sup_{\widetilde{V}:\|\widetilde{V}\|_{*} \leq 1/(1-\gamma)} |y^\top \widetilde{V}| \leq c_r/(1-\gamma).
    \end{align*}
    Now from the Lagragian duality we get, \begin{align*} \sigma_{{\Pp}} (V) &= QV +  \max_{\mu \geq 0, \alpha \in \R} \hspace{0.5cm} \min_{y\,:\,\sup_{\widetilde{V}:\|\widetilde{V}\|_{*} \leq 1/(1-\gamma)} |y^\top \widetilde{V}| \leq c_r/(1-\gamma)} \bigg( -Q\mu + y^\top (V-\mu-\alpha \mathbbm{1}) \bigg) \\
    &\stackrel{(a)}{=} QV +  \max_{V\geq \mu \geq 0, \alpha \in \R} \hspace{0.5cm} \min_{y\,:\,\sup_{\widetilde{V}:\|\widetilde{V}\|_{*} \leq 1/(1-\gamma)} |y^\top \widetilde{V}| \leq c_r/(1-\gamma)} \bigg( -Q\mu + y^\top (V-\mu-\alpha \mathbbm{1}) \bigg) \\
    &\stackrel{(b)}{=}  QV + \max_{V \geq \mu \geq 0, \alpha \in \R} \big( -Q\mu  - \min\{\| V-\mu-\alpha\mathbbm{1} \|_2^2, {c_r}/{(1-\gamma)}\}\big) \\
    &\stackrel{(c)}{=} QV + \max_{V \geq \mu \geq 0} \big( -Q\mu  - \min\{\| V-\mu-\alpha_\mu\mathbbm{1} \|_2^2, {c_r}/{(1-\gamma)}\}\big) ,
    \end{align*} where (a) follows from the complementary slackness condition. That is, if $\mu(s)>0$ for some $s\in\Ss$, then  from the complementary slackness condition we have that $y(s) = -Q(s)$. Now, if we further have  $\mu(s) > V(s)$ then \[  -Q(s)V(s)  + Q(s)\mu(s) \geq y(s) (V(s)-\mu(s)) \] \[  -Q(s)(V(s)   - \mu(s)) \geq y(s) (V(s)-\mu(s)) \]  \[  -Q(s)(\mu(s)   - V(s)) \geq y(s) (\mu(s)   - V(s)) \]
    $ -Q(s)V(s) = -Q(s)\mu(s) + y(s) (V(s)-\mu(s))$. Thus it suffices for the maximization over $\mu$ in range $V\geq \mu\geq 0.$
    (b) follows from Cauchy-Schwarz inequality and the condition $|y^\top \widetilde{V}| \leq c_r/(1-\gamma)$ for $\widetilde{V}=V-\mu-\alpha \mathbbm{1}$ satisfies $\|\widetilde{V}\|_{*} \leq 1/(1-\gamma)$ since $V-\mu \in [0,1/(1-\gamma)]^{|\Ss|}$, and (c) follows from calculus. This completes the proof.
\end{proof}
%%%% \mu <= V earlier inconsistency
% Notice that for all $\mu' > V$ we have $ -QV \geq -Q\mu' + y^\top (V-\mu')$ since $y\geq -Q$. With this note, now from the Lagragian duality we get, \begin{align*} \sigma_{{\Pp}} (V) &= QV +  \max_{V\geq \mu \geq 0, \alpha \geq 0} \hspace{0.5cm} \min_{y\,:\,\sup_{\widetilde{V}:\|\widetilde{V}\|_{*} \leq 1/(1-\gamma)} |y^\top \widetilde{V}| \leq c_r/(1-\gamma)} \bigg( -Q\mu + y^\top (V-\mu-\alpha \mathbbm{1}) \bigg) \\
%     &\stackrel{(a)}{=}  QV + \max_{V \geq \mu \geq 0, \alpha \geq 0} \big( -Q\mu  - \min\{\| V-\mu-\alpha\mathbbm{1} \|_2^2, {c_r}/{(1-\gamma)}\}\big) \\
%     &\stackrel{(b)}{=} QV + \max_{V \geq \mu \geq 0} \big( -Q\mu  - \min\{\| V-\mu-\alpha_\mu\mathbbm{1} \|_2^2, {c_r}/{(1-\gamma)}\}\big) ,
%     \end{align*} where (a) follows from Cauchy-Schwarz inequality and the condition $|y^\top \widetilde{V}| \leq c_r/(1-\gamma)$ for $\widetilde{V}=V-\mu-\alpha \mathbbm{1}$ satisfies $\|\widetilde{V}\|_{*} \leq 1/(1-\gamma)$ since $V-\mu \in [0,1/(1-\gamma)]^{|\Ss|}$ and (b) follows from calculus. This completes the proof of this lemma.
%%%% For IPM version:
% Now restating Lemma \ref{lem:ipm_inner_prob}.
% \begin{lemma}
%     Consider any ${V}\in \R^{|\Ss|}_+$. For an IPM-uncertainty set $\Pp$ centered with distribution $Q\in\Delta^{|\Ss|}$, \begin{align*} &\sigma_{{\Pp}} (V) = QV + \max_{\mu:0 \leq \mu \leq V} \big( -Q\mu  - \min\{\| V-\mu-\alpha_\mu\mathbbm{1} \|_2^2, {c_r}/{(1-\gamma)}\}\big),
%     \end{align*} where $\alpha_\mu = (1/|\Ss|)\sum_{s\in\Ss}(V(s)-\mu(s)).$
% \end{lemma}
% \begin{proof}
%     Recall the IPM-uncertainty set definition \[ \Pp =  \{ P \in \Delta^{|\Ss|} ~:~ \sup_{\widetilde{V}\in \R^{|\Ss|}} |P\widetilde{V} - Q\widetilde{V}| \leq c_r/(1-\gamma) \}. \] Letting $y(s) = P(s) - Q(s)$ for all $s\in\Ss$, we have \begin{align*} \sigma_{{\Pp}} (V) = QV + &\min && \hspace{-2cm} y^\top V  \\
%     &\text{s.t.} &&\hspace{-2cm}\sum_{s\in\Ss} y(s) = 0, y\geq -Q, \sup_{\widetilde{V}\in \R^{|\Ss|}} |y^\top \widetilde{V}| \leq c_r/(1-\gamma).
%     \end{align*}
%     From the Lagragian duality we get, \begin{align*} \sigma_{{\Pp}} (V) &= QV +  \max_{\mu \geq 0, \alpha \geq 0} \min_{y:\sup_{\widetilde{V}\in \R^{|\Ss|}} |y^\top \widetilde{V}| \leq c_r/(1-\gamma)} \bigg( -Q\mu + y^\top (V-\mu-\alpha \mathbbm{1}) \bigg) \\
%     &\stackrel{(a)}{=}  QV + \max_{\mu \geq 0, \alpha \in\R} \big( -Q\mu  - \min\{\| V-\mu-\alpha\mathbbm{1} \|_2^2, {c_r}/{(1-\gamma)}\}\big) \\
%     &\stackrel{(b)}{=} QV + \max_{\mu \geq 0} \big( -Q\mu  - \min\{\| V-\mu-\alpha_\mu\mathbbm{1} \|_2^2, {c_r}/{(1-\gamma)}\}\big) ,
%     \end{align*} where (a) follows from Cauchy-Schwarz inequality and the condition $|y^\top \widetilde{V}| \leq c_r/(1-\gamma)$ for $\widetilde{V}=V-\mu-\alpha \mathbbm{1} \in \R^{|\Ss|}$ and (b) follows from calculus. The proof is complete noting that ${V}\in \R^{|\Ss|}_+$ makes the optimal value of $\mu$ to satisfy $0 \leq \mu \leq V$.
% \end{proof}


Now restating Lemma \ref{lem:kl_inner_prob}.
\begin{lemma}[\hspace{-0.1cm}\text{\cite[Section 6.2]{nilim2005robust},\cite[Lemma 4.1]{iyengar2005robust}}]
    Consider any value function $V\in \R^{|\Ss|}$ bounded as $\|V\| \leq 1/(1-\gamma)$. For a KL-uncertainty set $\Pp$ centered with distribution $Q\in\Delta^{|\Ss|}$, \begin{align*} &\sigma_{{\Pp}} (V) = \max_{\lambda\in[0,\frac{1}{c_r(1-\gamma)}]} \bigg( -c_r \lambda  - \lambda \log (Q \exp(-V/\lambda)) \bigg), 
    \end{align*} where $\exp(-V/\lambda)$ is an element-wise exponential function. %and $c_{kl}$ is some positive constant defined as \begin{align*} c_{kl} = \inf \big\{ \lambda>0 ~:~ &\forall~ V'\in\R^{|\Ss|}\setminus\{0\}, \forall~ Q'\in\Delta^{|\Ss|},~ \\&c_r\lambda + \lambda\log(Q' \exp(-V'/\lambda)) + (1/Q' \exp(-V'/\lambda)) Q' (\exp(-V'/\lambda)V') = 0  \big\}, \end{align*} where $\exp(-V'/\lambda)V'$ is an element-wise product of vectors.
\end{lemma}
\begin{proof}
    This lemma directly follows from \cite[Section 6.2]{nilim2005robust} or \cite[Lemma 4.1]{iyengar2005robust}. It remains to show the upper bound for $\lambda$ in the optimization problem. Firstly, note that $-c_r \lambda  - \lambda \log (Q \exp(-V/\lambda))$ is concave in $\lambda$. Since $\sigma_{{\Pp}} (V) \geq 0$, for any $\lambda$ we have \begin{align*}
        0 &\leq -c_r \lambda  - \lambda \log (Q \exp(-V/\lambda)) \\
        &\stackrel{(a)}{\leq} -c_r \lambda  - \lambda \log ( \exp(-1/(\lambda(1-\gamma)))) \leq -c_r \lambda  - \frac{1}{1-\gamma},
    \end{align*} where (a) follows since $\|V\| \leq 1/(1-\gamma)$. %This concludes the upper bound of the range of $\lambda$ in the optimization problem. Now it remains to show the lower bound. This directly follows from calculus observing the first order condition of $-c_r \lambda  - \lambda \log (Q \exp(-V/\lambda))$ and noting that trivial solution for $\lambda$, that is $\lambda=0$, does not exist with $V\neq 0$. Now defining $c_{kl}$ as in the statement makes it an absolute positive constant. This completes the proof of this lemma.
\end{proof}


Now restating Lemma \ref{lem:sigma_probset_diff}.
\begin{lemma}
	%\label{lem:sigma_probset_diff}
	For some $\eta\in(0,1)$, define 
	\[ \begin{split} \widetilde{C}_{lw}(N,\eta) = &\frac{1}{1-\gamma}  \sqrt{\frac{\log(4|\Ss||\Aa|/\delta)}{2N}} +  2 \eta +  \frac{1}{1-\gamma} \sqrt{\frac{|\Ss|\log(6|\Ss||\Aa|/(\delta\eta(1-\gamma)))}{2N}}   . \end{split}\]
	Consider any value function $V\in \R^{|\Ss|}$ bounded as $\|V\| \leq 1/(1-\gamma)$. Then, for both $\ell_1$ and Wasserstein uncertainty sets, \[\max_{s,a}| \sigma_{\widehat{\Pp}_{s,a}} (V) - \sigma_{{\Pp}_{s,a}} (V)  | \leq   \widetilde{C}_{lw}(N,\eta)\] holds with probability at least $1-\delta$. 
\end{lemma}
\begin{proof}
	Fix any $(s,a)$ pair. %From \cite[Lemma 4.3]{iyengar2005robust} we have that \begin{align*}
% 	    &\sigma_{{\Pp}_{s,a}} (V) = P^o_{s,a} V + \frac{c_r}{2} \cdot \\&\hspace{0.5cm}\max_{\mu: 0 \leq \mu \leq V} \bigg( -P^o_{s,a} \mu - \max_{s} (V_\mu(s)) + \min_{s} (V_\mu(s)) \bigg) \\
% 	    &\sigma_{\widehat{\Pp}_{s,a}} (V) = \widehat{P}_{s,a} V + \frac{c_r}{2} \cdot \\&\hspace{0.5cm} \max_{\mu: 0 \leq \mu \leq V} \bigg( -\widehat{P}_{s,a} \mu - \max_{s} (V_\mu(s)) + \min_{s} (V_\mu(s)) \bigg),
% 	\end{align*} where $0\leq\mu\leq V$ is an elementwise inequality and $V_\mu(s)=V(s)-\mu(s)$ for all $s\in\Ss$.
	For both $\ell_1$ and Wasserstein uncertainty sets from Lemmas \ref{lem:l1_inner_prob} and \ref{lem:wasserstein_inner_prob}, with the additional fact that $|\max_{x} f(x)-\max_{x} g(x)| \leq \max_{x} |f(x) - g(x)|$, we have \[ \begin{split} &| \sigma_{\widehat{\Pp}_{s,a}} (V) - \sigma_{{\Pp}_{s,a}} (V)  | \leq | \widehat{P}_{s,a} V - P^o_{s,a} V| + \max_{\mu: 0 \leq \mu \leq V} | \widehat{P}_{s,a} \mu - P^o_{s,a} \mu|. \end{split} \] 
	
	Note that $\|\mu\| \leq \|V\| \leq 1/(1-\gamma)$. Fix some $\mu\in\V$ and $\eta\in(0,1)$. From $\N_\V$, we know that there exists $\mu'\in\N_\V$ such that $\sup_{s\in\Ss} |\mu(s)-\mu'(s)| \leq \eta$.  Thus, \begin{align*}
	    | \widehat{P}_{s,a} \mu - P^o_{s,a} \mu| &\leq | \widehat{P}_{s,a} \mu' - P^o_{s,a} \mu'| + | \widehat{P}_{s,a} (\mu-\mu')|  + | P^o_{s,a} (\mu-\mu')| \\
	    &\stackrel{(a)}{\leq} | \widehat{P}_{s,a} \mu' - P^o_{s,a} \mu'| + \| \widehat{P}_{s,a}\|_1 \|\mu-\mu'\| + \| P^o_{s,a}\|_1 \|\mu-\mu'\| \\
	   % &\leq | \widehat{P}_{s,a} \mu' - P^o_{s,a} \mu'| + 2\eta \\
	    &\leq \sup_{\mu'\in\N_\V} \max_{s,a}| \widehat{P}_{s,a} \mu' - P^o_{s,a} \mu'| + 2\eta \\
	    &\stackrel{(b)}{\leq} \frac{1}{1-\gamma} \sqrt{\frac{\log(2|\Ss||\Aa|\N_\eta/\delta)}{2N}} + 2\eta \\
	    &\stackrel{(c)}{\leq} \frac{1}{1-\gamma} \sqrt{\frac{|\Ss|\log(6|\Ss||\Aa|/(\delta\eta(1-\gamma)))}{2N}} + 2\eta,
	    %&\stackrel{(d)}{=} \frac{1}{1-\gamma} \sqrt{\frac{|\Ss|\log(12|\Aa|N/(\delta(1-\gamma)))}{2N}}  + \frac{|\Ss|}{N},
	\end{align*} where (a) follows from H$\ddot{\text{o}}$lder's inequality, (b) from Lemma \ref{lem:hoeffding_concentration}, and (c) from Lemma \ref{por:covering_num}. %, and (d) by choosing $\eta=|\Ss|/(2N)$. %\redtext{Actually, optimal $\eta=\eta^*$ satisfies \[ \eta^* = \frac{|\Ss|}{4(1-\gamma)\sqrt{2N}\sqrt{\log(\frac{2|\Ss||\Aa|}{\delta}(\frac{3}{\eta^*})^{|\Ss|})}}. \]} 
	Finally, we have with probability at least $1-\delta/2$, \[ \begin{split}
	&\max_{s,a}| \sigma_{\widehat{\Pp}_{s,a}} (V) - \sigma_{{\Pp}_{s,a}} (V)  | \leq \max_{s,a} | \widehat{P}_{s,a} V - P^o_{s,a} V| +  \frac{1}{1-\gamma} \sqrt{\frac{|\Ss|\log(6|\Ss||\Aa|/(\delta\eta(1-\gamma)))}{2N}}  + {2\eta}. \end{split}\] Again, using the union bound and Lemma \ref{lem:hoeffding_concentration} completes the proof. 
\end{proof}

Now restating Lemma \ref{lem:sigma_probset_diff_chisquared}.
\begin{lemma}
% 	\label{lem:sigma_probset_diff_chisquared}
	For some $\eta\in(0,\min\{1, (1-l_\chi)^2/(4(1-\gamma)) \})$ where $l_\chi\in(0,1)$, define 
	\[ \begin{split} &\widetilde{C}_{\chi}(N,\eta) = (1+\sqrt{c_r})\,\widetilde{C}_{lw}(N,\eta) + \eta\sqrt{c_r} + \frac{\sqrt{2 c_r}}{(1-\gamma)l_\chi} \sqrt{\frac{|\Ss|\log(6|\Ss||\Aa|/(\delta\eta(1-\gamma)))}{N}} + \frac{4\sqrt{\eta c_r}}{\sqrt{1-\gamma}} . \end{split}\]
	Consider any value function $V\in [l_\chi/(1-\gamma), 1/(1-\gamma)]^{|\Ss|}$. Then, for the $\chi^2$ uncertainty set, \[\max_{s,a}| \sigma_{\widehat{\Pp}_{s,a}} (V) - \sigma_{{\Pp}_{s,a}} (V)  | \leq   \widetilde{C}_{\chi}(N,\eta)\] holds with probability at least $1-\delta$. 
\end{lemma}
\begin{proof}
	Fix any $(s,a)$ pair. {For the $\chi^2$ uncertainty set from Lemma \ref{lem:chi2_inner_prob},} with the additional facts that $|\max_{x} f(x)-\max_{x} g(x)| \leq \max_{x} |f(x) - g(x)|$ and $\max_{x} f(x)+g(x) \leq \max_{x} f(x)+\max_{x} g(x)$, we have \[ \begin{split} | \sigma_{\widehat{\Pp}_{s,a}} (V) - \sigma_{{\Pp}_{s,a}} (V)  | &\leq \max_{\mu: 0 \leq \mu \leq V} | \widehat{P}_{s,a} (V-\mu) - P^o_{s,a} (V-\mu)| \\&\hspace{1cm}+ \max_{\mu: 0 \leq \mu \leq V} | \sqrt{c_r \text{Var}_{\widehat{P}_{s,a}}(V-\mu)} - \sqrt{c_r \text{Var}_{P^o_{s,a}}(V-\mu)}|. \end{split} \] 
	From the analysis in Lemma \ref{lem:sigma_probset_diff}, it is enough to analyze the third term above.
	
	Fix some $\mu\in\V$. Let $c_r \text{Var}_{\widehat{P}_{s,a}}(V-\mu) \geq c_r \text{Var}_{P^o_{s,a}}(V-\mu)$. We now have \begin{align*}
	  &0 \leq \sqrt{c_r \text{Var}_{\widehat{P}_{s,a}}(V-\mu)} - \sqrt{c_r \text{Var}_{P^o_{s,a}}(V-\mu)} \\
	  &\stackrel{(a)}{\leq} \sqrt{c_r} | \sqrt{ \widehat{P}_{s,a}(V-\mu)^2} - \sqrt{P^o_{s,a}(V-\mu)^2}| + \sqrt{c_r}  |P^o_{s,a}(V-\mu) - \widehat{P}_{s,a}(V-\mu)| ,
	\end{align*} where (a) follows since $\sqrt{|a-b|} \leq \sqrt{a} + \sqrt{b}$ for all $a,b\geq 0$. Following the same procedure for $c_r \text{Var}_{\widehat{P}_{s,a}}(V-\mu) \leq c_r \text{Var}_{P^o_{s,a}}(V-\mu)$, we finally get \begin{align*}
	   |\sqrt{c_r \text{Var}_{\widehat{P}_{s,a}}(V-\mu)} - \sqrt{c_r \text{Var}_{P^o_{s,a}}(V-\mu)}| &\leq  \sqrt{c_r} | \sqrt{ \widehat{P}_{s,a}(V-\mu)^2} - \sqrt{P^o_{s,a}(V-\mu)^2}| \\&\hspace{1cm}+ \sqrt{c_r}  |P^o_{s,a}(V-\mu) - \widehat{P}_{s,a}(V-\mu)| .
	\end{align*}
	
	Now fix some $\eta\in(0,\min\{1, (1-l_\chi)^2/(4(1-\gamma)) \})$. From $\N_\V$, we know that there exists $\mu'\in\N_\V$ such that $\sup_{s\in\Ss} |\mu(s)-\mu'(s)| \leq \eta$. Let $\widehat{P}_{s,a} (V-\mu)^2 \geq P^o_{s,a} (V-\mu)^2$. We now have \begin{align*}
	    0 \leq  \sqrt{\widehat{P}_{s,a} (V-\mu)^2} - \sqrt{P^o_{s,a} (V-\mu)^2} &=
	    \sqrt{\widehat{P}_{s,a} ((V-\mu')^2 + (\mu-\mu')^2 + 2(V-\mu')\circ(\mu'-\mu))}  \\
	    &- \sqrt{{P}^o_{s,a} ((V-\mu')^2 + (\mu-\mu')^2 + 2(V-\mu')\circ(\mu'-\mu))}  \\
	    &\stackrel{(a)}{\leq}  \sqrt{\widehat{P}_{s,a} (V-\mu')^2} + \eta + \frac{2\sqrt{\eta}}{\sqrt{1-\gamma}}  \\
	    &- \sqrt{{P}^o_{s,a} ((V-\mu')^2 + (\mu-\mu')^2 + 2(V-\mu')\circ(\mu'-\mu))}  \\
	    &\stackrel{(b)}{\leq} \sqrt{\widehat{P}_{s,a} (V-\mu')^2} - \sqrt{{P}^o_{s,a} (V-\mu')^2} + \eta + \frac{4\sqrt{\eta}}{\sqrt{1-\gamma}} \\
	    &{\leq} |\sqrt{\widehat{P}_{s,a} (V-\mu')^2} - \sqrt{{P}^o_{s,a} (V-\mu')^2} | + \eta + \frac{4\sqrt{\eta}}{\sqrt{1-\gamma}} \\
	    &\stackrel{(c)}{\leq} \frac{\sqrt{2}}{(1-\gamma)l_\chi} \sqrt{\frac{\log(2|\Ss||\Aa|\N_\eta/\delta)}{N}} + \eta + \frac{4\sqrt{\eta}}{\sqrt{1-\gamma}} \\
	    &\stackrel{(d)}{\leq} \frac{\sqrt{2}}{(1-\gamma)l_\chi} \sqrt{\frac{|\Ss|\log(6|\Ss||\Aa|/(\delta\eta(1-\gamma)))}{N}} + \eta + \frac{4\sqrt{\eta}}{\sqrt{1-\gamma}} ,
	\end{align*} where (a) follows from  $\sup_{s\in\Ss} |\mu(s)-\mu'(s)| \leq \eta$ and $\sup_{s\in\Ss}(V(s)-\mu'(s))(\mu'(s)-\mu(s)) \leq 2\eta/(1-\gamma)$ in lieu of the fact $\sqrt{a+b} \leq \sqrt{a} + \sqrt{b}$ for all $a,b\geq 0$, 
	(b) follows from $\inf_{s\in\Ss}(V(s)-\mu'(s))(\mu'(s)-\mu(s)) \geq -2\eta/(1-\gamma)$ and $\inf_{s\in\Ss} |V(s)-\mu'(s)| \geq (1-l_\chi)/(1-\gamma)$ in lieu of the fact $\sqrt{c-d} \geq \sqrt{c} - \sqrt{d}$ for all $c\geq d\geq 0$,
	(c) holds with high probability following the analysis in Lemma \ref{lem:hoeffding_concentration} with the additional fact that $\{ \sqrt{\widehat{P}_{s,a} (V-\mu')^2} - \sqrt{{P}^o_{s,a} (V-\mu')^2} > \epsilon \} \subseteq \{ {\widehat{P}_{s,a} (V-\mu')^2} - {{P}^o_{s,a} (V-\mu')^2} > 2\epsilon l_\chi / (1-\gamma) \} $,
	and (d) from Lemma \ref{por:covering_num}.
	
	Finally we have, \[ \begin{split}
	\max_{s,a}| \sigma_{\widehat{\Pp}_{s,a}} (V) - \sigma_{{\Pp}_{s,a}} (V)  | \leq \eta \sqrt{c_r} &+ (1+\sqrt{c_r}) \max_{s,a} \max_{\mu: 0 \leq \mu \leq V} | \widehat{P}_{s,a} (V-\mu) - P^o_{s,a} (V-\mu)| 
	\\&+\frac{\sqrt{2 c_r}}{(1-\gamma)l_\chi} \sqrt{\frac{|\Ss|\log(6|\Ss||\Aa|/(\delta\eta(1-\gamma)))}{N}} + \frac{4\sqrt{\eta c_r}}{\sqrt{1-\gamma}}. \end{split}\] Now following the steps in Lemma \ref{lem:sigma_probset_diff} proof for the second summation above completes the proof of this lemma. 
\end{proof}

\redtext{
\begin{lemma}[\redtext{Sub-optimal but correct result for $\chi^2$ uncertainty set}]
	\label{lem:}
	For some $\eta\in(0,1)$, define 
	\[ \begin{split} &\widetilde{C}_{\chi}(N,\eta) = c\,\widetilde{C}_{li}(N,\eta) + \\&\hspace{0.2cm}+  \frac{2\sqrt{c_r}c}{(1-\gamma)} \bigg(\frac{|\Ss|\log(6|\Ss||\Aa|/(\delta\eta(1-\gamma)))}{2N}\bigg)^{1/4} + \sqrt{2c\,c_r}\eta \\&\hspace{4cm}+   \sqrt{\frac{8c\, c_r\eta}{1-\gamma}} , \end{split}\] where $c>0$ is some absolute constant.
	Consider any value function $V\in \R^{|\Ss|}$ bounded as $\|V\| \leq 1/(1-\gamma)$. Then, for the $\chi^2$ uncertainty set, \[\max_{s,a}| \sigma_{\widehat{\Pp}_{s,a}} (V) - \sigma_{{\Pp}_{s,a}} (V)  | \leq   \widetilde{C}_{\chi}(N,\eta)\] holds with probability at least $1-\delta$. 
\end{lemma}
\begin{proof}
	Fix any $(s,a)$ pair. \bluetext{For the $\chi^2$ uncertainty set,} with the additional facts that $|\max_{x} f(x)-\max_{x} g(x)| \leq \max_{x} |f(x) - g(x)|$ and $\max_{x} f(x)+g(x) \leq \max_{x} f(x)+\max_{x} g(x)$, we have \[ \begin{split} &| \sigma_{\widehat{\Pp}_{s,a}} (V) - \sigma_{{\Pp}_{s,a}} (V)  | \leq \\&\max_{\mu: 0 \leq \mu \leq V} | \widehat{P}_{s,a} (V-\mu) - P^o_{s,a} (V-\mu)| \\&\hspace{0cm}+ \max_{\mu: 0 \leq \mu \leq V} | \sqrt{c_r \text{Var}_{\widehat{P}_{s,a}}(V-\mu)} - \sqrt{c_r \text{Var}_{P^o_{s,a}}(V-\mu)}|. \end{split} \] 
	From the analysis in Lemma \ref{lem:sigma_probset_diff}, it is enough to analyze the third term above.
	
	Fix some $\mu\in\V$. Let $c_r \text{Var}_{\widehat{P}_{s,a}}(V-\mu) \geq c_r \text{Var}_{P^o_{s,a}}(V-\mu)$. We now have \begin{align*}
	  &0 \leq \sqrt{c_r \text{Var}_{\widehat{P}_{s,a}}(V-\mu)} - \sqrt{c_r \text{Var}_{P^o_{s,a}}(V-\mu)} \\
	  &\stackrel{(a)}{\leq} \sqrt{c_r \text{Var}_{\widehat{P}_{s,a}}(V-\mu) -c_r \text{Var}_{P^o_{s,a}}(V-\mu)} \\
	  &\stackrel{(b)}{\leq} \sqrt{c_r |\widehat{P}_{s,a}(V-\mu)^2 - P^o_{s,a}(V-\mu)^2|} \\&\hspace{0.5cm}+ \sqrt{c_r |(P^o_{s,a}(V-\mu))^2 - (\widehat{P}_{s,a}(V-\mu))^2| }\\
	  &\stackrel{(c)}{\leq} \sqrt{c_r |\widehat{P}_{s,a}(V-\mu)^2 - P^o_{s,a}(V-\mu)^2|} \\&\hspace{0.5cm}+ \sqrt{\frac{2 c_r}{1-\gamma}} \sqrt{ |P^o_{s,a}(V-\mu) - \widehat{P}_{s,a}(V-\mu)| },
	\end{align*} where (a), (b) follows since $\sqrt{a+b} \leq \sqrt{a} + \sqrt{b}$ for all $a,b\geq 0$, and (c) follows from Holder's inequality and the fact that $\|\mu\| \leq \|V\| \leq 1/(1-\gamma)$. Following the same procedure for $c_r \text{Var}_{\widehat{P}_{s,a}}(V-\mu) \leq c_r \text{Var}_{P^o_{s,a}}(V-\mu)$, we finally get \begin{align*}
	   &|\sqrt{c_r \text{Var}_{\widehat{P}_{s,a}}(V-\mu)} - \sqrt{c_r \text{Var}_{P^o_{s,a}}(V-\mu)}| \leq \\ &\sqrt{c_r |\widehat{P}_{s,a}(V-\mu)^2 - P^o_{s,a}(V-\mu)^2|} \\&\hspace{0.5cm}+ \sqrt{\frac{2 c_r}{1-\gamma}} \sqrt{ |P^o_{s,a}(V-\mu) - \widehat{P}_{s,a}(V-\mu)| }.
	\end{align*}
	
	Now fix some $\eta\in(0,1)$. From $\N_\V$, we know that there exists $\mu'\in\N_\V$ such that $\sup_{s\in\Ss} |\mu(s)-\mu'(s)| \leq \eta$.  Thus, \begin{align*}
	    &| \widehat{P}_{s,a} (V-\mu)^2 - P^o_{s,a} (V-\mu)^2| \leq \\
	    &| \widehat{P}_{s,a} (V-\mu')^2 - P^o_{s,a} (V-\mu')^2| \\
	    &+ | \widehat{P}_{s,a} (\mu-\mu')^2 - P^o_{s,a} (\mu-\mu')^2|  \\&\hspace{0.2cm}+ 2| \widehat{P}_{s,a} (V-\mu')\circ(\mu'-\mu) - P^o_{s,a} (V-\mu')\circ(\mu'-\mu)| \\
	    &\stackrel{(a)}{\leq} | \widehat{P}_{s,a} (V-\mu')^2 - P^o_{s,a} (V-\mu')^2| + 2\eta^2 + \frac{8\eta}{1-\gamma} \\
	    &\leq \sup_{\mu'\in\N_\V} \max_{s,a} | \widehat{P}_{s,a} (V-\mu')^2 - P^o_{s,a} (V-\mu')^2| + 2\eta^2 \\&\hspace{4cm}+  \frac{8\eta}{1-\gamma}  \\
	    &\stackrel{(b)}{\leq} \frac{4}{(1-\gamma)^2} \sqrt{\frac{\log(2|\Ss||\Aa|\N_\eta/\delta)}{2N}} +  2\eta^2 +  \frac{8\eta}{1-\gamma}  \\
	    &\stackrel{(c)}{\leq} \frac{4}{(1-\gamma)^2} \sqrt{\frac{|\Ss|\log(6|\Ss||\Aa|/(\delta\eta(1-\gamma)))}{2N}} + 2\eta^2 \\&\hspace{4cm}+   \frac{8\eta}{1-\gamma} ,
	    %&\stackrel{(d)}{=} \frac{1}{1-\gamma} \sqrt{\frac{|\Ss|\log(12|\Aa|N/(\delta(1-\gamma)))}{2N}}  + \frac{|\Ss|}{N},
	\end{align*} where (a) follows from H$\ddot{\text{o}}$lder's inequality, (b) from Lemma \ref{lem:hoeffding_concentration} with $V_{\max}={4}/{(1-\gamma)^2}$,  and (c) from Lemma \ref{por:covering_num}.
	Finally we have, \[ \begin{split}
	&\max_{s,a}| \sigma_{\widehat{\Pp}_{s,a}} (V) - \sigma_{{\Pp}_{s,a}} (V)  | \leq \\&\max_{s,a} \max_{\mu: 0 \leq \mu \leq V} | \widehat{P}_{s,a} (V-\mu) - P^o_{s,a} (V-\mu)| 
	\\&+\sqrt{\frac{2 c_r}{1-\gamma}} \max_{s,a} \max_{\mu: 0 \leq \mu \leq V} \sqrt{| \widehat{P}_{s,a} (V-\mu) - P^o_{s,a} (V-\mu)|}
	\\&\hspace{0.2cm}+  \frac{2\sqrt{c_r}}{(1-\gamma)} \bigg(\frac{|\Ss|\log(6|\Ss||\Aa|/(\delta\eta(1-\gamma)))}{2N}\bigg)^{1/4} + \sqrt{2c_r}\eta \\&\hspace{4cm}+   \sqrt{\frac{8 c_r\eta}{1-\gamma}}. \end{split}\] Now following the steps in Lemma \ref{lem:sigma_probset_diff} proof for the first two terms above completes the proof of this lemma. 
\end{proof}

}


Now restating Lemma \ref{lem:sigma_probset_diff_KL}.
\begin{lemma}
% 	\label{lem:sigma_probset_diff_KL}
	Define 
	\[ \begin{split} \widetilde{C}_{kl}(N) = \frac{1}{c_r(1-\gamma)} \cdot \exp(\frac{1}{c_{kl}(1-\gamma)}) \sqrt{\frac{\log(6|\Ss||\Aa|/\delta)}{2N}}. \end{split}\]
	Let $N$ satisfy \begin{align} \label{eq:kl_N_cond}
	    N \geq {2\log(2|\Ss||\Aa|/\delta)} \exp(\frac{2}{c_{kl}(1-\gamma)}).
	\end{align}
	Consider any value function $V\in \R^{|\Ss|}_+$ bounded as $\|V\| \leq 1/(1-\gamma)$. Then, for the KL uncertainty set, \[\max_{s,a}| \sigma_{\widehat{\Pp}_{s,a}} (V) - \sigma_{{\Pp}_{s,a}} (V)  | \leq   \widetilde{C}_{kl}(N)\] holds with probability at least $1-\delta$. 
\end{lemma}
\begin{proof}
	Fix any $(s,a)$ pair.
	\redtext{For the KL uncertainty set from Lemma \ref{lem:kl_inner_prob}, we have \begin{align*} &\sigma_{{\Pp}_{s,a}} (V) = \max_{\lambda\in[0,\frac{1}{c_r(1-\gamma)}]} \bigg( -c_r \lambda  - \lambda \log (P^o_{s,a} \exp(-V/\lambda)) \bigg), \\
	&\sigma_{\widehat{\Pp}_{s,a}} (V) = \max_{\lambda\in[0,\frac{1}{c_r(1-\gamma)}]} \bigg( -c_r \lambda  - \lambda \log (\widehat{P}_{s,a} \exp(-V/\lambda)) \bigg).
    \end{align*}
    
    From \cite{nilim2005robust} it follows that whenever the maximizer $\lambda$ is $0$, we have $\sigma_{{\Pp}_{s,a}} (V) = V_{\min}$ and $\sigma_{\widehat{\Pp}_{s,a}} (V) = V_{\min}$ where $V_{\min}=\min_{j\in\Ss} V(j)$.
    
    Let \begin{align*} &\lambda^* \in \argmax_{\lambda\in[0,\frac{1}{c_r(1-\gamma)}]} \bigg( -c_r \lambda  - \lambda \log (P^o_{s,a} \exp(-V/\lambda)) \bigg), \\
	&\widehat{\lambda}^* \in \argmax_{\lambda\in[0,\frac{1}{c_r(1-\gamma)}]} \bigg( -c_r \lambda  - \lambda \log (\widehat{P}_{s,a} \exp(-V/\lambda)) \bigg).
    \end{align*} From \cite[Lemma 4 (1)]{zhou2021finite}, we have that if $\lambda^*=0$, then with probability at least $1-\delta/(3|\Ss||\Aa|)$ we have $\widehat{\lambda}^*=0$ for $N\geq N'(\delta/(3|\Ss||\Aa|), c_r, P^o_{s,a})$ [DEFINED IN \cite{zhou2021finite}, need to write it here].
    
    Thus, whenever $\lambda^*=0$, we have $| \sigma_{\widehat{\Pp}_{s,a}} (V) - \sigma_{{\Pp}_{s,a}} (V)  | = |V_{\min} - V_{\min}| = 0$, with probability at least $1-\delta/(3|\Ss||\Aa|)$.
    
    Again from \cite[Lemma 4 (2)]{zhou2021finite}, if $\lambda^* \in [\underline{\lambda},{1}/{(c_r(1-\gamma))}]$ for some $\underline{\lambda}>0$ independent of $N$, then with probability at least $1-\delta/(3|\Ss||\Aa|)$ we have $\widehat{\lambda}^*\in [\underline{\lambda},{1}/{(c_r(1-\gamma))}]$ for $N\geq N''(\delta/(3|\Ss||\Aa|), c_r, P^o_{s,a})$ [DEFINED IN \cite{zhou2021finite}, need to write it here].
	
	So, whenever  $\lambda^* \in [\underline{\lambda},{1}/{(c_r(1-\gamma))}]$ we have
	 \begin{align*} &\sigma_{{\Pp}_{s,a}} (V) = \max_{\lambda\in[\underline{\lambda},\frac{1}{c_r(1-\gamma)}]} \bigg( -c_r \lambda  - \lambda \log (P^o_{s,a} \exp(-V/\lambda)) \bigg), \\
	&\sigma_{\widehat{\Pp}_{s,a}} (V) = \max_{\lambda\in[\underline{\lambda},\frac{1}{c_r(1-\gamma)}]} \bigg( -c_r \lambda  - \lambda \log (\widehat{P}_{s,a} \exp(-V/\lambda)) \bigg).
    \end{align*}
    }
    
	Now with the additional fact that $|\max_{x} f(x)-\max_{x} g(x)| \leq \max_{x} |f(x) - g(x)|$, we have \[ \begin{split} &| \sigma_{\widehat{\Pp}_{s,a}} (V) - \sigma_{{\Pp}_{s,a}} (V)  | \leq  \max_{\lambda\in[\underline{\lambda},\frac{1}{c_r(1-\gamma)}]} | \lambda \log (\frac{P^o_{s,a} \exp(-V/\lambda)}{ \widehat{P}_{s,a} \exp(-V/\lambda) } )|. \end{split} \]
	
	Using the upper bound for $\lambda$ and rearranging we have \begin{align} &| \sigma_{\widehat{\Pp}_{s,a}} (V) - \sigma_{{\Pp}_{s,a}} (V)  | \leq \frac{1}{c_r(1-\gamma)} \cdot \label{eq:kl_main_1}  \max_{\lambda\in[\underline{\lambda},\frac{1}{c_r(1-\gamma)}]} |  \log (1 + \frac{(P^o_{s,a}- \widehat{P}_{s,a}) \exp(-V/\lambda) }{ \widehat{P}_{s,a} \exp(-V/\lambda) } )|.  \end{align}
	
	We now deviate to show a high probability result that is useful in our analysis. \begin{align*}
	    \frac{|(P^o_{s,a}- \widehat{P}_{s,a}) \exp(-V/\lambda)| }{| \widehat{P}_{s,a} \exp(-V/\lambda) |} &\stackrel{(a)}{\leq} \frac{|(P^o_{s,a}- \widehat{P}_{s,a}) \exp(-V/\lambda)| }{\exp(\frac{-1}{\underline{\lambda}(1-\gamma)})} \\
	    &\stackrel{(b)}{\leq} \exp(\frac{1}{\underline{\lambda}(1-\gamma)}) \sqrt{\frac{\log(6|\Ss||\Aa|/\delta)}{2N}},
	\end{align*} where (a) follows since $\lambda\geq \underline{\lambda}$ and $\|V\|\leq 1/(1-\gamma)$, and (b) follows from Lemma \ref{lem:hoeffding_concentration} with $V_{\max}=1$ since $V\in\R^{\Ss}_+$. Using this in \eqref{eq:kl_main_1}, under the condition \eqref{eq:kl_N_cond} and the fact $|\log(1+x)| \leq |x|$ for $|x|\leq 1/2$, we have 
	\begin{align*} &| \sigma_{\widehat{\Pp}_{s,a}} (V) - \sigma_{{\Pp}_{s,a}} (V)  | \leq \frac{1}{c_r(1-\gamma)} \cdot  \exp(\frac{1}{\underline{\lambda}(1-\gamma)}) \sqrt{\frac{\log(6|\Ss||\Aa|/\delta)}{2N}}. \end{align*}
	This completes the proof of this lemma. 
\end{proof}

Now restating Lemma \ref{lem:sigma_v_diff}.
\begin{lemma}
% 	\label{lem:sigma_v_diff}
	For any $(s,a)\in\ScA$ and  for any $ V_{1}, V_{2} \in \R^{|\Ss|}$,
	\begin{align*}
	    |{\sigma}_{{\Pp}_{s,a}} (V_{1}) - {\sigma}_{{\Pp}_{s,a}} (V_{2}) | \leq \|V_{1} - V_{2}\| \text{ and }
	     |{\sigma}_{\widehat{\Pp}_{s,a}} (V_{1}) - {\sigma}_{\widehat{\Pp}_{s,a}} (V_{2}) | \leq \|V_{1} - V_{2}\|.
	\end{align*}
\end{lemma}
\begin{proof}
	We only prove the first inequality since the proof is analogous for the other inequality. For any $(s,a)\in\ScA$ we have  
	\begin{align}
	 \sigma_{{{\Pp}_{s,a}}} (V_2) - \sigma_{{{\Pp}_{s,a}}} (V_1) &= \hspace{-0.2cm} \inf_{q \in {{\Pp}_{s,a}}} q^\top V_2 - \inf_{\tilde{q} \in {{\Pp}_{s,a}}} \tilde{q}^\top V_1 \nonumber \\
	&= \inf_{q \in {{\Pp}_{s,a}} } \sup_{\tilde{q} \in {{\Pp}_{s,a}}} q^\top V_2 - \tilde{q}^\top V_1 \nonumber  \\
	&\geq \inf_{q \in {{\Pp}_{s,a}} } q^\top (V_2 - V_1) = \sigma_{{\Pp}_{s,a}} (V_2 - V_1).
	\label{eq:lemma_sigma_d-1}
	\end{align} By definition, for any arbitrary $\epsilon > 0$, there exists a $P_{s,a}  \in \Pp_{s,a} $ such that
	\begin{align}
	\label{eq:lemma_sigma_d-2}
	P^{\top}_{s,a} (V_{2} - V_{1}) - \epsilon \leq \sigma_{{\Pp_{s,a}}} (V_2 - V_1).
	\end{align}
	Using \eqref{eq:lemma_sigma_d-2} and \eqref{eq:lemma_sigma_d-1},
	\begin{align*}
	 \sigma_{{{\Pp}_{s,a}}} (V_1) - \sigma_{{{\Pp}_{s,a}}} (V_2)  &\leq  P^{\top}_{s,a}  (V_{1} - V_{2}) +  \epsilon \leq  P^{\top}_{s,a}  |(V_{2} - V_{1})| +  \epsilon \\
	&\stackrel{(a)}{\leq}    \|P_{s,a}\|_1  \|V_{1} - V_{2}\|  +  \epsilon
	=    \|V_{1} - V_{2}\|  +  \epsilon
	\end{align*}
	where $(a)$ follows from Holder's inequality. Since $\epsilon$ is arbitrary, we get, $\sigma_{{{\Pp}_{s,a}}} (V_1) - \sigma_{{{\Pp}_{s,a}}} (V_2)  \leq   \|V_{1} - V_{2}\| $. Exchanging the roles of $V_1$ and $V_2$ completes the proof.
\end{proof}
%%%% Vectorized version of the above lemma:
% \begin{lemma}
% 	\label{lem:sigma_v_diff}
% 	For any policy $\pi$, ${\sigma}_{{\Pp}_\pi}$ and ${\sigma}_{\widehat{\Pp}_\pi}$ are $1$-Lipschitz functions, that is, for any $ V_{1}, V_{2} \in \R^{|\Ss|}$,
% 	$\|{\sigma}_{{\Pp}_\pi} (V_{1}) - {\sigma}_{{\Pp}_\pi} (V_{2}) \| \leq \|V_{1} - V_{2}\| $ and $ \|{\sigma}_{\widehat{\Pp}_\pi} (V_{1}) - {\sigma}_{\widehat{\Pp}_\pi} (V_{2}) \| \leq \|V_{1} - V_{2}\|.$
% \end{lemma}
% \begin{proof}
% 	We only prove the first inequality since the proof is analogous for the other inequality. For any $\pi$ and $s\in\Ss$ we have  
% 	\begin{align}
% 	& \sigma_{{{\Pp}_{s,\pi(s)}}} (V_2) - \sigma_{{{\Pp}_{s,\pi(s)}}} (V_1) = \hspace{-0.2cm} \inf_{q \in {{\Pp}_{s,\pi(s)}}} q^\top V_2 - \inf_{\tilde{q} \in {{\Pp}_{s,\pi(s)}}} \tilde{q}^\top V_1 \nonumber \\
% 	&= \inf_{q \in {{\Pp}_{s,\pi(s)}} } \sup_{\tilde{q} \in {{\Pp}_{s,\pi(s)}}} q^\top V_2 - \tilde{q}^\top V_1 \nonumber  \\
% 	&\geq \inf_{q \in {{\Pp}_{s,\pi(s)}} } q^\top (V_2 - V_1) = \sigma_{{\Pp}_{s,\pi(s)}} (V_2 - V_1).
% 	\label{eq:lemma_sigma_d-1}
% 	\end{align} By definition, for any arbitrary $\epsilon > 0$, there exists a $P_{s, \pi(s)}  \in \Pp_{s, \pi(s)} $ such that
% 	\begin{align}
% 	\label{eq:lemma_sigma_d-2}
% 	P^{\top}_{s, \pi(s)} (V_{2} - V_{1}) - \epsilon \leq \sigma_{{\Pp_{s,\pi(s)}}} (V_2 - V_1).
% 	\end{align}
% 	Using \eqref{eq:lemma_sigma_d-2} and \eqref{eq:lemma_sigma_d-1},
% 	\begin{align*}
% 	 &\sigma_{{{\Pp}_{s,\pi(s)}}} (V_1) - \sigma_{{{\Pp}_{s,\pi(s)}}} (V_2)  \leq  P^{\top}_{s, \pi(s)}  (V_{1} - V_{2}) +  \epsilon\\
% 	&\leq  P^{\top}_{s, \pi(s)}  |(V_{2} - V_{1})| +  \epsilon \\
% 	&\stackrel{(b)}{\leq}    \|P_{s, \pi(s)}\|_1  \|V_{1} - V_{2}\|  +  \epsilon
% 	=    \|V_{1} - V_{2}\|  +  \epsilon
% 	\end{align*}
% 	where $(b)$ follows from Holder's inequality. Since $\epsilon$ is arbitrary, we get, $\sigma_{{{\Pp}_{s,\pi(s)}}} (V_1) - \sigma_{{{\Pp}_{s,\pi(s)}}} (V_2)  \leq   \|V_{1} - V_{2}\| $. Exchanging roles of $V_1$ and $V_2$ completes the proof.
% \end{proof}

We now present an intermediate result that is used in the proof of Theorems \ref{thm:revi-guarantee-l1-Wasserstein}-\ref{thm:revi-guarantee-kul-lieb}. We define an approximate robust Bellman operator $ \widehat{T} (V) (s) =  \max_{a} ( r(s,a) + \gamma \sigma_{\widehat{\Pp}_{s,a}}(V(s'))).$ Similar to the operator $T$, it is known  \cite{iyengar2005robust} that $\widehat{T}$ is a contraction in sup norm. Let $\widehat{V}^{*}$ be the unique fixed point of $\widehat{T}$. The following proposition shows that $\widehat{V}^{*}$ approximates the true optimal robust value $V^*$ with high probability. We also let ${\hat{\pi}^*}$ be the optimal policy for the operator $\widehat{T}$. For notational convenience, for any policy $\pi$ we define $\widehat{Q}^{\pi}(s,a) = r(s,a) + \gamma \sigma_{\widehat{\Pp}_{s,a}}(\widehat{V}^{\pi}(s'))$ and ${Q}^{\pi}(s,a) = r(s,a) + \gamma \sigma_{{\Pp}_{s,a}}({V}^{\pi}(s'))$. We note that since $|r(s,a)|\leq 1$ for all $(s,a)\in\ScA$, $\|{V}^{\pi}\| \leq \| {Q}^{\pi}\| \leq 1/(1-\gamma)$ and $\|\widehat{V}^{\pi}\| \leq \| \widehat{Q}^{\pi}\| \leq 1/(1-\gamma)$ for any $\pi.$ Finally, we use $\widetilde{C}(N,\eta)$ to denote $\widetilde{C}_{lw}(N,\eta)$ or $\widetilde{C}_{\chi}(N,\eta)$ or $\widetilde{C}_{kl}(N)$ until we make it explicit.

Now restating Proposition \ref{prop:optimal_robust_value_bound}.
\begin{proposition}%\label{prop:optimal_robust_value_bound}
	Fix $\delta\in(0,1)$. Under Assumption 1, the following holds with probability at least $1-\delta$, \[\| V^* - \widehat{V}^* \| \leq \frac{\gamma}{1-\gamma} \cdot  \widetilde{C}(N,\eta),\] where $\eta$ is any value in $(0,1)$. 
\end{proposition}
\begin{proof}
	For $s\in\Ss$, \begin{align*}
	V^*(s) -  \widehat{V}^{*}(s) &= Q^*(s,\pi^*(s)) -  \widehat{Q}^*(s,\hat{\pi}^*(s)) \\
	&\stackrel{(a)}{\leq}  Q^*(s,\pi^*(s)) -  \widehat{Q}^*(s,\pi^*(s)) \\	
	&\stackrel{(b)}{=} \gamma \sigma_{{\Pp}_{s,\pi^*(s)}} (V^*) - \gamma \sigma_{\widehat{\Pp}_{s,\pi^*(s)}} (\widehat{V}^*)\\
	&= \gamma  (\sigma_{{\Pp}_{s,\pi^*(s)}} (V^*) -  \sigma_{{\Pp}_{s,\pi^*(s)}} (\widehat{V}^*) +  \sigma_{{\Pp}_{s,\pi^*(s)}} (\widehat{V}^*) - \sigma_{\widehat{\Pp}_{s,\pi^*(s)}} (\widehat{V}^*) )\\
	&\stackrel{(c)}{\leq}  \gamma \|V^*-\widehat{V}^{*}\| + \gamma\, \widetilde{C}(N,\eta) ,
	\end{align*} where (a) follows since ${\hat{\pi}^*}$ is the robust optimal policy for $\widehat{T}$, (b) follows from the definitions of $Q^*$ and $\widehat{Q}^*$, and (c) follows from Lemma \ref{lem:sigma_v_diff} and Lemma \ref{lem:sigma_probset_diff}.
	
	Similarly, we get \[  \widehat{V}^{*}(s) -  V^*(s) \leq \gamma \|V^*-\widehat{V}^{*}\| + \gamma\,  \widetilde{C}(N,\eta). \] 
Now taking max w.r.t $s$ on both sides in the above equation, we get \[ \|V^*-\widehat{V}^{*}\| \leq  \gamma \|V^*-\widehat{V}^{*}\| +  \gamma\,  \widetilde{C}(N,\eta). \] Rearranging, we get  \[ \|V^*-\widehat{V}^{*}\| \leq  \frac{\gamma}{1-\gamma} \cdot \widetilde{C}(N,\eta). \]
This completes the proof.
\end{proof}

Now restating Lemma \ref{lem:singh_yee_main_result}.
\begin{lemma}%\label{lem:singh_yee_main_result}
    \[ \| \widehat{V}^{*} - \widehat{V}^{\pi_k} \| \leq \frac{2\gamma}{1-\gamma} \| V_k  - \widehat{V}^{*} \| .  \]
\end{lemma}
\begin{proof}
    The proof is analogous to the proof in \cite{singh1994upper} in addition to, by Lemma \ref{lem:sigma_v_diff}, ${\sigma}_{\widehat{\Pp}_{s,a}}$ being a $1$-Lipschitz function for any $(s,a)\in\ScA$. %$\|{\sigma}_{\widehat{\Pp}_\pi} (V_{1}) - {\sigma}_{\widehat{\Pp}_\pi} (V_{2}) \| \leq \|V_{1} - V_{2}\|$.
\end{proof}
% \begin{proof}
%     Fix any state $s\in\Ss$. We have \begin{align*}
%         \widehat{V}^{*}(s) - \widehat{V}^{\pi_k}(s) &=   \widehat{Q}^*(s,\hat{\pi}^*(s)) -  \widehat{Q}^{\pi_k}(s,\pi_k(s)) \\
%         &=   \widehat{Q}^*(s,\hat{\pi}^*(s)) - \widehat{Q}^*(s,\pi_k(s)) + \widehat{Q}^*(s,\pi_k(s)) - \widehat{Q}^{\pi_k}(s,\pi_k(s)) \\
%         &=   \widehat{Q}^*(s,\hat{\pi}^*(s)) - \widehat{Q}^*(s,\pi_k(s)) + \gamma \sigma_{\widehat{\Pp}_{s,\pi_k(s)}} (\widehat{V}^{*}) - \gamma \sigma_{\widehat{\Pp}_{s,\pi_k(s)}} (\widehat{V}^{\pi_k})  \\
%         &\stackrel{(a)}{\leq} \widehat{Q}^*(s,\hat{\pi}^*(s)) - \widehat{Q}^*(s,\pi_k(s)) + \gamma \| \widehat{V}^{*} - \widehat{V}^{\pi_k} \|  \\
%         &\stackrel{(b)}{\leq} \widehat{Q}^*(s,\hat{\pi}^*(s)) - Q_k(s,\hat{\pi}^*(s)) + Q_k(s,\pi_k(s)) - \widehat{Q}^*(s,\pi_k(s)) + \gamma \| \widehat{V}^{*} - \widehat{V}^{\pi_k} \|  \\&\leq 2 \| Q_k  - \widehat{Q}^* \| + \gamma \| \widehat{V}^{*} - \widehat{V}^{\pi_k} \|,
%     \end{align*} where (a) follows from Lemma 7 and (b) from the fact that $\pi_k$ is greedy w.r.t $Q_k$'s. Similarly we have \begin{align*}
%         \widehat{V}^{\pi_k}(s) - \widehat{V}^{*}(s)  &=   \widehat{Q}^{\pi_k}(s,\pi_k(s)) - \widehat{Q}^*(s,\hat{\pi}^*(s))   \\
%         &\stackrel{(a)}{\leq}  \widehat{Q}^{\pi_k}(s,\pi_k(s)) - \widehat{Q}^*(s,\pi_k(s)) 
%         \\
%         &= \widehat{Q}^*(s,\hat{\pi}^*(s)) - \widehat{Q}^*(s,\pi_k(s)) + \widehat{Q}^*(s,\pi_k(s)) - \widehat{Q}^{\pi_k}(s,\pi_k(s)) \\
%         &=   \widehat{Q}^*(s,\hat{\pi}^*(s)) - \widehat{Q}^*(s,\pi_k(s)) + \gamma \sigma_{\widehat{\Pp}_{s,\pi_k(s)}} (\widehat{V}^{*}) - \gamma \sigma_{\widehat{\Pp}_{s,\pi_k(s)}} (\widehat{V}^{\pi_k})  \\
%         &\stackrel{(a)}{\leq} \widehat{Q}^*(s,\hat{\pi}^*(s)) - \widehat{Q}^*(s,\pi_k(s)) + \gamma \| \widehat{V}^{*} - \widehat{V}^{\pi_k} \|  \\
%         &\stackrel{(b)}{\leq} \widehat{Q}^*(s,\hat{\pi}^*(s)) - Q_k(s,\hat{\pi}^*(s)) + Q_k(s,\pi_k(s)) - \widehat{Q}^*(s,\pi_k(s)) + \gamma \| \widehat{V}^{*} - \widehat{V}^{\pi_k} \|  \\&\leq 2 \| Q_k  - \widehat{Q}^* \| + \gamma \| \widehat{V}^{*} - \widehat{V}^{\pi_k} \|,
%     \end{align*} where (a) follows from Lemma 7 and (b) from the fact that $\pi_k$ is greedy w.r.t $Q_k$'s.
%     This completes the proof.
% \end{proof}

	
\begin{proof}[\textbf{Proof of Theorems \ref{thm:revi-guarantee-l1-Wasserstein}-\ref{thm:revi-guarantee-kul-lieb}}]
	In lieu of the triangle inequality \[ \| V^* - V^{\pi_k} \| \leq \| V^* - \widehat{V}^{*} \| + \| \widehat{V}^{*} - \widehat{V}^{\pi_k} \| + \| \widehat{V}^{\pi_k} - V^{\pi_k} \| \] and Proposition \ref{prop:optimal_robust_value_bound}, it is enough to bound the last two terms in the above inequality.
	
	For all $k \geq 1$, since $\widehat{T}$ is $\gamma$-contraction, we have \begin{align*}
	\|Q_k -  \widehat{Q}^*\| 
	= \|\widehat{T}Q_{k-1} -  \widehat{T} \widehat{Q}^*\|
	\leq \gamma \|Q_{k-1} -  \widehat{Q}^*\|.
	\end{align*} From the recursion, we get \[ \|Q_k -  \widehat{Q}^*\| \leq \gamma^k \|Q_{0} -  \widehat{Q}^*\| = \gamma^k \|\widehat{Q}^*\| \leq \frac{\gamma^k}{1-\gamma}. \] Noting that $\|V_k -  \widehat{V}^{*}\| \leq \|Q_k -  \widehat{Q}^*\| $, we have $ \| V_k  - \widehat{V}^{*} \| \leq {\gamma^k}/{(1-\gamma)}.$ Thus, from Lemma \ref{lem:singh_yee_main_result} it follows that \[ \| \widehat{V}^{*} - \widehat{V}^{\pi_k} \| \leq \frac{2\gamma^{k+1}}{(1-\gamma)^2}.  \]
	To bound $\| \widehat{V}^{\pi_k} - V^{\pi_k} \|$, we follow the proof in Proposition \ref{prop:optimal_robust_value_bound}. For $s\in\Ss$, \begin{align*}
	V^{\pi_k}(s) -  \widehat{V}^{\pi_k}(s) &=   Q^{\pi_k}(s,\pi_k(s)) -  \widehat{Q}^{\pi_k}(s,\pi_k(s)) \\	&\stackrel{(a)}{=} \gamma \sigma_{{\Pp}_{s,\pi_k(s)}} (V^{\pi_k}) - \gamma \sigma_{\widehat{\Pp}_{s,\pi_k(s)}} (\widehat{V}^{\pi_k})\\
	&= \gamma  (\sigma_{{\Pp}_{s,\pi_k(s)}} (V^{\pi_k}) -  \sigma_{{\Pp}_{s,\pi_k(s)}} (\widehat{V}^{\pi_k}) +  \sigma_{{\Pp}_{s,\pi_k(s)}} (\widehat{V}^{\pi_k}) - \sigma_{\widehat{\Pp}_{s,\pi_k(s)}} (\widehat{V}^{\pi_k}) )\\
	&\stackrel{(b)}{\leq}  \gamma \|V^{\pi_k}-\widehat{V}^{\pi_k}\| + \gamma\, \widetilde{C}(N,\eta),
	\end{align*} where (a) follows from the definitions of $Q^{\pi_k}$ and $\widehat{Q}^{\pi_k}$, and (b) follows from Lemma \ref{lem:sigma_v_diff} and Lemma \ref{lem:sigma_probset_diff}.
	
	Similarly, we get \[  \widehat{V}^{\pi_k}(s) -  V^{\pi_k}(s) \leq \gamma \|V^{\pi_k}-\widehat{V}^{\pi_k}\| + \gamma \, \widetilde{C}(N,\eta). \] 
Now taking max w.r.t $s$ on both sides in the above equation, we get \[ \|V^{\pi_k}-\widehat{V}^{\pi_k}\| \leq  \gamma \|V^{\pi_k}-\widehat{V}^{\pi_k}\| +  \gamma\,  \widetilde{C}(N,\eta). \] Rearranging, we get  \[ \|V^{\pi_k}-\widehat{V}^{\pi_k}\| \leq  \frac{\gamma}{1-\gamma} \cdot \widetilde{C}(N,\eta). \]


% l1 and IPM
For the Assumptions 1.1 or 1.2, i.e. Wasserstein or $\ell_1$ uncertainty sets respectively, we use $\widetilde{C}_{lw}(N,\eta)$ for $\widetilde{C}(N,\eta)$. Then, with probability at least $1-2\delta$, we finally have \[ \begin{split} \| V^* - V^{\pi_k} \| \leq &\frac{2\gamma^{k+1}}{(1-\gamma)^2} + \frac{2\gamma}{(1-\gamma)^2}   \sqrt{\frac{\log(4|\Ss||\Aa|/\delta)}{2N}} \\& +  \frac{4\gamma \eta}{(1-\gamma)}  + \frac{2\gamma}{(1-\gamma)^2}  \sqrt{\frac{|\Ss|\log(6|\Ss||\Aa|/(\delta\eta(1-\gamma)))}{2N}}   . \end{split} \]
We now choose $\eta=\epsilon(1-\gamma)/(16\gamma )$. Since $\epsilon\in(0,16\gamma /(1-\gamma))$, this particular $\eta$ is in $(0,1)$. Now we get $\| V^* - V^{\pi_k} \|\leq \epsilon$ when $k$ and $N$ satisfy the conditions \eqref{eq:li_Wasserstein_conditions}. This completes the proof of Theorem \ref{thm:revi-guarantee-l1-Wasserstein}.

% chi^2
For the Assumption 1.3, i.e. $\chi^2$ uncertainty set, we use $\widetilde{C}_{\chi}(N,\eta)$ for $\widetilde{C}(N,\eta)$. Then, with probability at least $1-2\delta$, we finally have \[ \begin{split} \| V^* - V^{\pi_k} \| \leq \frac{2\gamma^{k+1}}{(1-\gamma)^2} &+ \frac{2c\gamma}{(1-\gamma)^2}   \sqrt{\frac{\log(4|\Ss||\Aa|/\delta)}{2N}} \\& +  \frac{4c\gamma \eta}{1-\gamma}  + \frac{2c\gamma}{(1-\gamma)^2}  \sqrt{\frac{|\Ss|\log(6|\Ss||\Aa|/(\delta\eta(1-\gamma)))}{2N}}  \\&+
\frac{2\eta\sqrt{c_r}\gamma}{1-\gamma} + \frac{8\gamma\sqrt{\eta c_r}}{(1-\gamma)^{1.5}}  \\&+ \frac{2\gamma\sqrt{2 c_r}}{(1-\gamma)^2 l_\chi} \sqrt{\frac{|\Ss|\log(6|\Ss||\Aa|/(\delta\eta(1-\gamma)))}{N}} , \end{split} \] where $c=(1+\sqrt{c_r})$.
We now choose $\eta=\epsilon(1-\gamma)/(16\gamma )$. Since $\epsilon\in(0,16\gamma /(1-\gamma))$, this particular $\eta$ is in $(0,1)$. Now we get $\| V^* - V^{\pi_k} \|\leq \epsilon$ when $k$ and $N$ satisfy the conditions \eqref{eq:chi_conditions}.  This completes the proof of Theorem \ref{thm:revi-guarantee-chi2}.

% KL
For the Assumption 1.4, i.e. KL uncertainty set, we use $\widetilde{C}_{kl}(N,\eta)$ for $\widetilde{C}(N,\eta)$. Then, with probability at least $1-2\delta$, we finally have \[ \begin{split} \| V^* - V^{\pi_k} &\| \leq \frac{2\gamma^{k+1}}{(1-\gamma)^2} + \frac{2\gamma}{c_r(1-\gamma)^2} \cdot \exp(\frac{1}{c_{kl}(1-\gamma)}) \sqrt{\frac{\log(2|\Ss||\Aa|/\delta)}{2N}}. \end{split} \]
Now we get $\| V^* - V^{\pi_k} \|\leq \epsilon$ when $k$ and $N$ satisfy the conditions \eqref{eq:kl_conditions}. This completes the proof of Theorem \ref{thm:revi-guarantee-kul-lieb}.
\end{proof}


% \begin{proof}[\textbf{Proof of Corollary \ref{thm:corollary}}] Suppose $k$ satisfies the given condition, then we have ${2\gamma^{k+1}}/{(1-\gamma)^2} \leq \epsilon/4$. Now, for any $\eta\in(0,1)$, from the proof of Theorem \ref{thm:robust_guarantee_rtvi} we have
% \[ \begin{split} &\| V^* - V^{\pi_k} \| \leq \frac{\epsilon}{4} + \frac{2\gamma}{(1-\gamma)^2}   \sqrt{\frac{\log(4|\Ss||\Aa|/\delta)}{2N}} \\& +  \frac{2\gamma c_r \eta}{(1-\gamma)}  + \frac{c_r}{2} \frac{2\gamma}{(1-\gamma)^2}  \sqrt{\frac{|\Ss|\log(6|\Ss||\Aa|/(\delta\eta(1-\gamma)))}{2N}}   . \end{split} \]
% %% log N version
% % \[ \begin{split} &\| V^* - V^{\pi_k} \| \leq \frac{\epsilon}{4} +  \frac{2\gamma}{(1-\gamma)^2} \sqrt{\frac{\log(4|\Ss||\Aa|/\delta)}{2N}} \\&+ \frac{c_r\gamma}{(1-\gamma)^2} \sqrt{\frac{|\Ss|\log(24|\Aa|N/(\delta(1-\gamma)))}{2N}}  + \frac{c_r\gamma|\Ss|}{(1-\gamma)2N}. \end{split} \] 
% We now choose $\eta=\epsilon(1-\gamma)/(8\gamma c_r)$. Since $\epsilon\in(0,8\gamma c_r/(1-\gamma))$, this particular $\eta$ is in $(0,1)$. We have the required bound when $N$ satisfies the given condition.   
% \end{proof}

\section{Proof of Theorem \ref{thm:non-robust-policy-suboptimality}}


\begin{proof}
    We consider the deterministic  MDP $(\Ss, \Aa, r, P^o, \gamma)$ shown in Fig.\ref{fig:chain-mdp-nominal} to be the nominal model. We fix $\gamma\in(0.01,1]$ and $s_1=0$. The state space is $\Ss = \{0,1\}$ and action space is $\Aa = \{a_{l}, a_{r}\},$ where $a_{l}$ denotes `move left' and $a_{r}$ denotes `move right' action. Reward for state $1$ and action $a_r$ pair is $r(1, a_{r}) = 1$, for state $0$ and action $a_r$ pair is $r(0, a_{r}) = -100\gamma/99$, and the reward is $0$ for all other $(s,a)$. Transition function $P^{o}$ is deterministic, as indicated by the arrows. 
\begin{figure}[ht]
	\centering
	\includegraphics[width=0.5\linewidth]{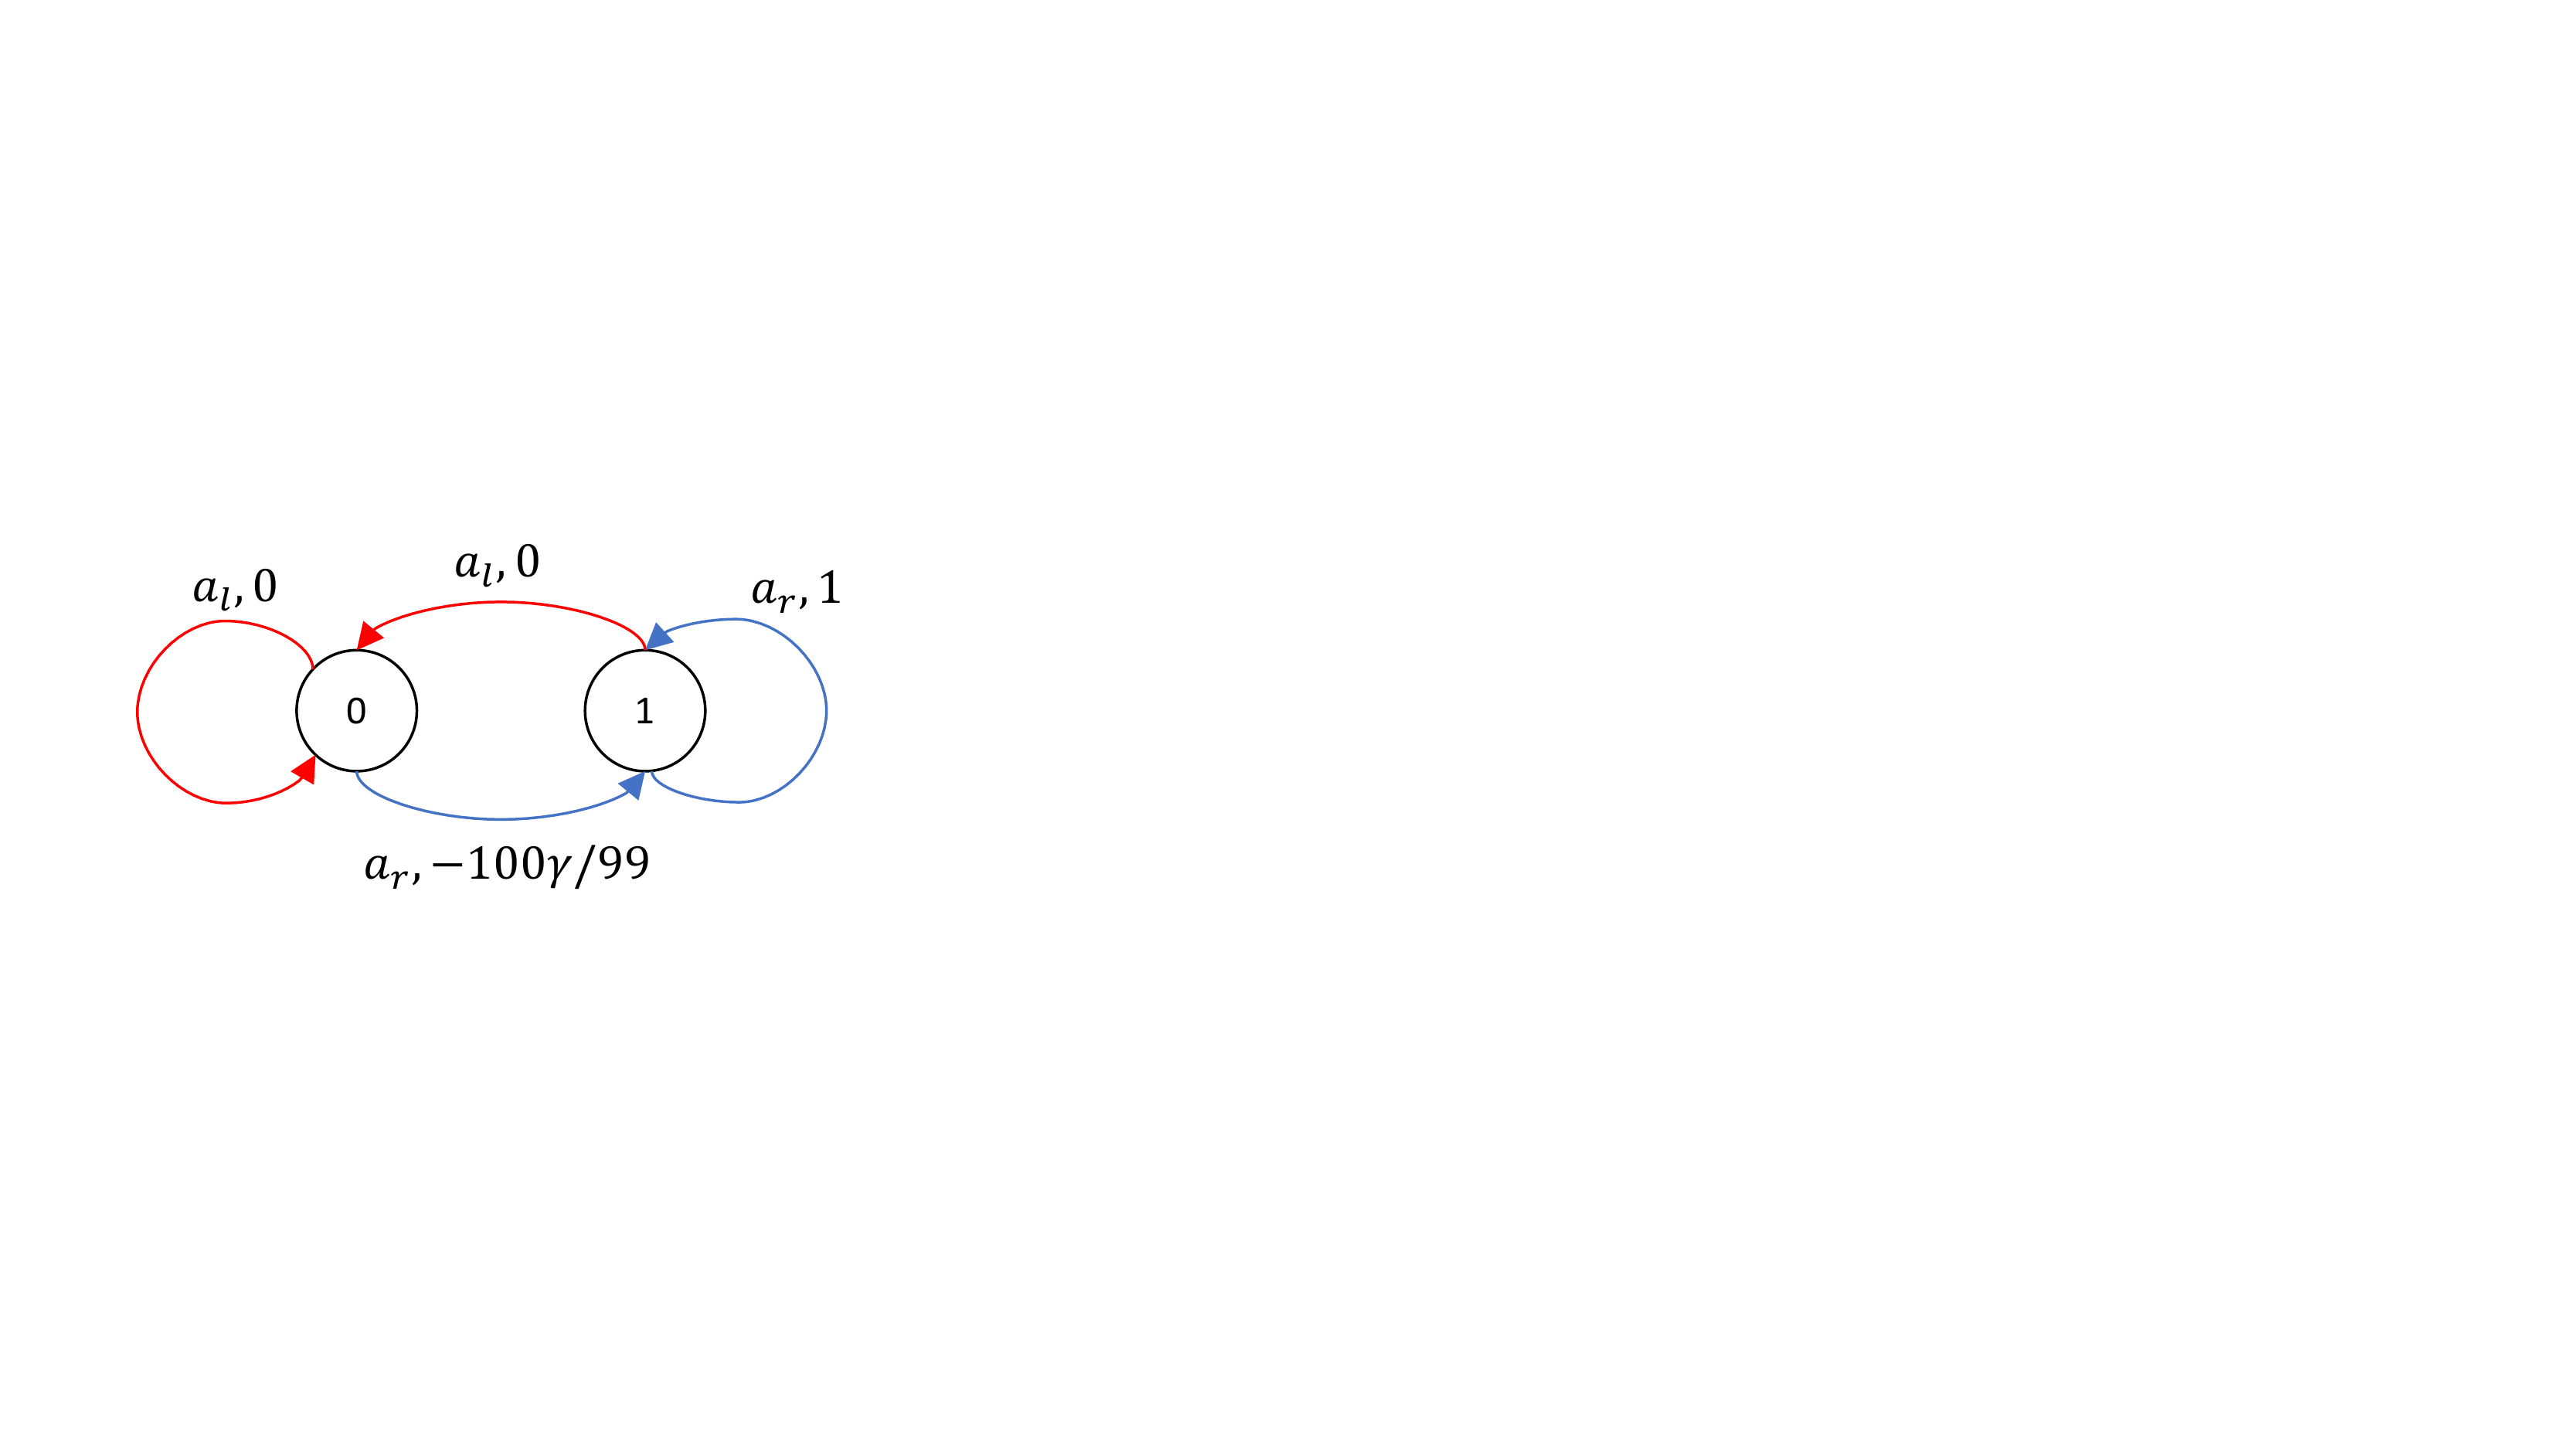}
	\captionof{figure}{Transitions and rewards corresponding to the nominal model $P^o$. The states $\{0,1\}$ are given inside the circles, and the actions $\{a_l,a_r\}$ and  associated  rewards are given on the corresponding  transitions.}
	\label{fig:chain-mdp-nominal}
\end{figure}

Similarly, we consider another deterministic model $P'$, as shown in Fig.\ref{fig:chain-mdp-p}. We consider the set $\Pp=\{P^o,P'\}$. 
 \begin{figure}[ht]
	\centering
	\includegraphics[width=0.5\linewidth]{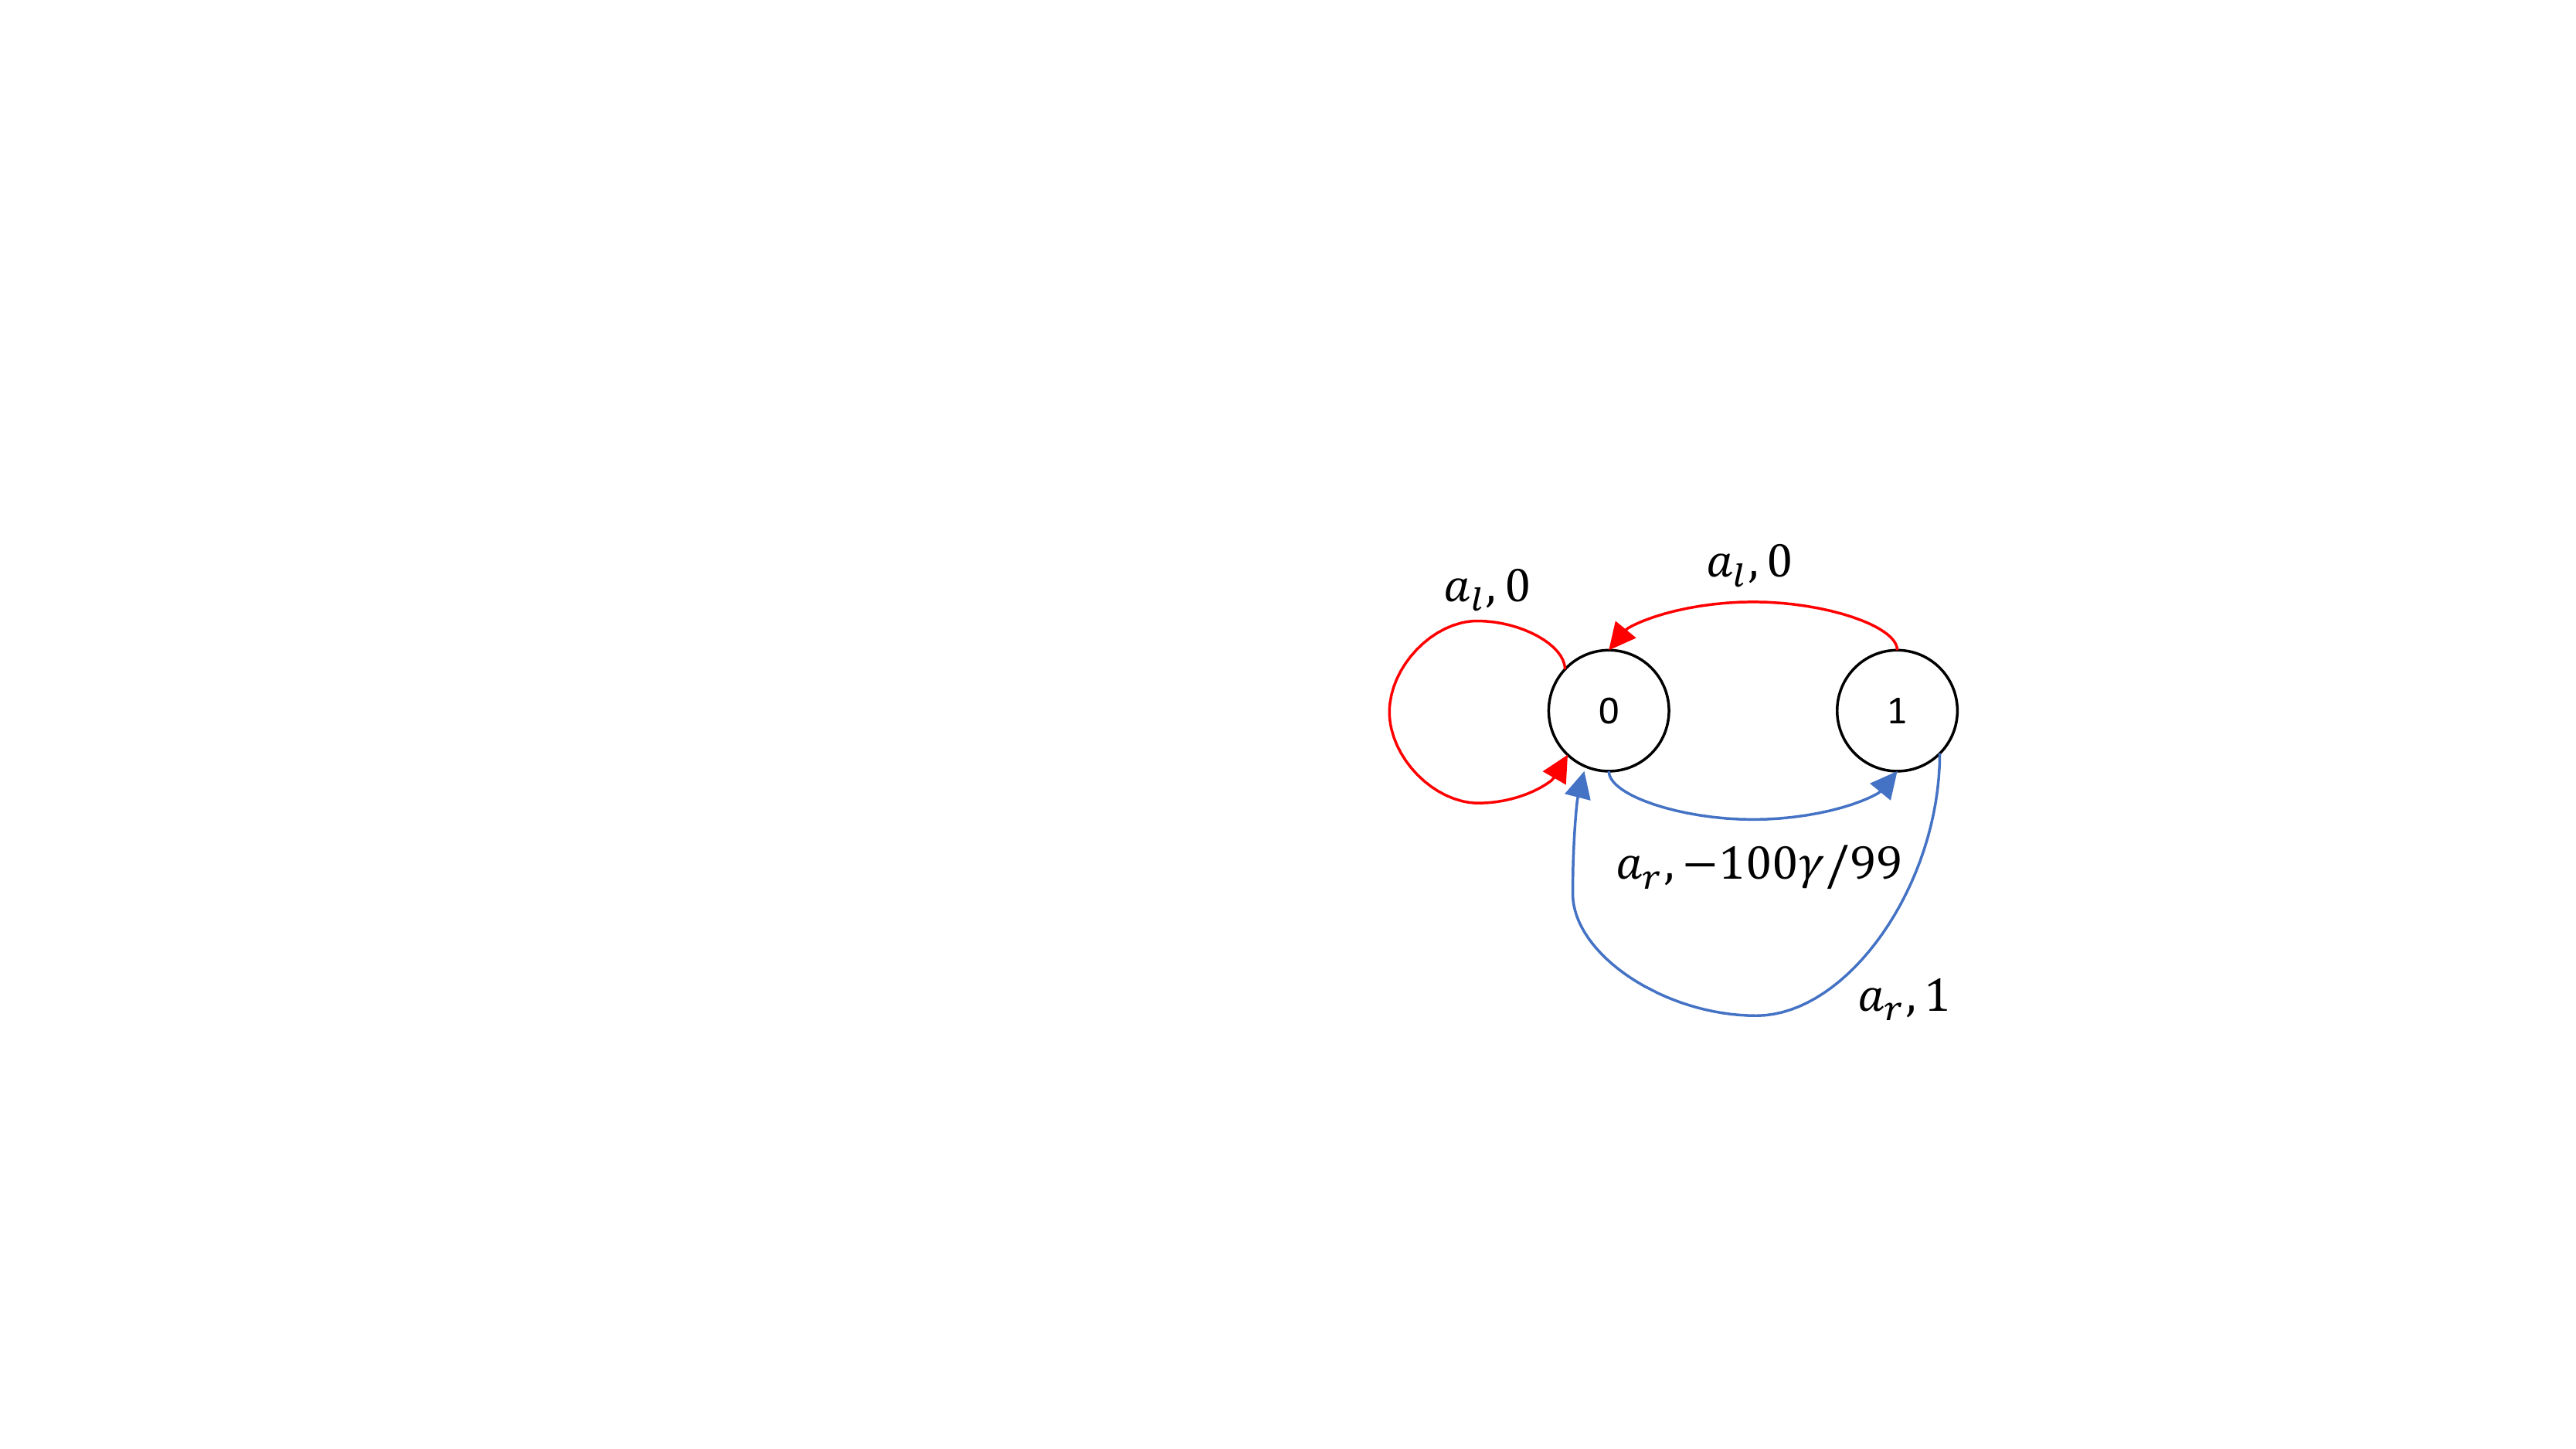}
	\captionof{figure}{Transitions and rewards corresponding to the model $P'$.}
	\label{fig:chain-mdp-p}
    \end{figure}

    It is straight forward to show that taking action $a_r$ in any state  is the optimal non-robust policy $\pi^{o}$ corresponding to the nominal model $P^{o}$. This is obvious if for state $s=1$. For $s = 0$, notice that taking action $a_{l}$ will give a value zero and taking action $a_{r}$ will give a value  $\frac{\gamma}{1-\gamma} - \frac{100\gamma}{99}$. Since $\gamma > 0.01$, taking action $a_{r}$ will give a positive value and hence  is optimal. So, we get 
    \[V_{{\pi}^{o},P^o}(0) = \frac{\gamma}{1-\gamma} - \frac{100\gamma}{99}.\]
    
    Similarly, it is  straightforward to see that taking the action $a_l$ at each state  is the optimal non-robust policy $\pi'$ corresponding to the  model $P'$, which will give the value $V_{\pi', P'}(0) = 0$. 
    
    
    We can now compute $V_{{\pi}^{o},P'}(0)$ using the recursive equation
    \[ V_{{\pi}^{o},P'}(0) = - \frac{100\gamma}{99} + \gamma + \gamma^2 V_{{\pi}^{o},P'}(0). \] 
    Solving this, we get $V_{{\pi}^{o},P'}(0) = -\gamma/(99(1-\gamma^2))$. 
    
    Now the robust value of $\pi^{o}$ is given by
    \begin{align*}
        V^{{\pi}^{o}}(s) = \min\{V_{{\pi}^{o},P^o}(0),V_{{\pi}^{o},P'}(0)\} = -\gamma/(99(1-\gamma^2)). 
    \end{align*}
    
  
    % Thus, the robust value for the policy $\bar{\pi}^*$ is $\min\{V_{\bar{\pi}^*,P'}(s_1=0),V_{\bar{\pi}^*,P^o}(s_1=0)\}.$ It is straightforward to see that taking deterministic action $a_r$ at every time gives us the optimal non-robust value for $P^o$. Thus, we have that \[V_{\bar{\pi}^*,P^o}(s_1=0) = \frac{\gamma}{1-\gamma} - \frac{100\gamma}{99} = \frac{100\gamma^2 - \gamma}{99(1-\gamma)} > 0,\] where the strict inequality follows since $\gamma\in(0.01,1]$. Since the policy $\bar{\pi}^*$ is taking action $a_r$ at every state, we get the following recursive equation: \[ V_{\bar{\pi}^*,P'}(s_1=0) = - \frac{100\gamma}{99} + \gamma + \gamma^2 V_{\bar{\pi}^*,P'}(s_1=0). \] Solving this we get $V_{\bar{\pi}^*,P'}(s_1=0)=-\gamma/(99(1-\gamma^2)).$ Thus, $V^{\bar{\pi}^*}(s_1=0) = -\gamma/(99(1-\gamma^2))$.
    
    Now, we find the optimal robust value $V^{*}(0)$. From the perfect duality result of robust MDP \cite[Theorem 1]{nilim2005robust}, we have
    \begin{align*}
        V^*(0) &= \min \{\max_\pi V_{\pi,P^o}(0), \max_\pi V_{\pi,P'}(0)\} \\
        &= \min \{V_{{\pi}^{o},P^o}(0),  V_{\pi', P'}(0)\} = 0. 
    \end{align*}
    
    
    % $V^*(s_1=0) = \min \{ \max_\pi V_{\pi,P'}(s_1=0), \max_\pi V_{\pi,P^o}(s_1=0) \}.$ It is straightforward to see that taking deterministic action $a_l$ at every time gives us the maximum value of $V_{\pi,P'}(s_1=0)$, which is $0$. Noticing that $\max_\pi V_{\pi,P^o}(s_1=0) = V_{\bar{\pi}^*,P^o}(s_1=0)$, we have $V^*(s_1=0)=0$.
    
    We finally have \begin{align*}
        V^*(0) - V^{{\pi}^{o}}(0) = \frac{\gamma}{99(1-\gamma^2)} \geq \frac{\gamma}{198(1-\gamma)},
    \end{align*} where the inequality follows since $1+\gamma\leq2$. Thus, setting $c=\gamma/198$ and $\gamma_o=0.01$, completes the proof of this theorem.
\end{proof}
